# Supplementary material for: Interacting Mathieu equation, synchronization dynamics and collision-induced velocity exchange in trapped ions
Source: arXiv:2406.12306 source file (2024-06-18)
Supplement: Supplementary file 1 [file appendix.tex]

\section{Appendix}
